# Supplementary material for: Feature Extractor or Decision Maker: Rethinking the Role of Visual Encoders in Visuomotor Policies
Source: arXiv:2409.20248 source file (2025-05-14)
Supplement: Supplementary file 1 [file supplementary.tex]

\section{Full Related Work}
%%%%%%%%%%%%%%%%%%%%%%%%%%%%%%%%%%%%%%%%%%%%%%%%%%%%%%%%%%%%%%%%%%
\textbf{Robotic Visuomotor Policy.}
Current BC approaches can be categorized into two groups: explicit policy and implicit policy. Explicit policy forms the simplest version of BC by directly regressing the action or control signals through current environmental observation \citep{NIPS1988_812b4ba2, RahmatizadehABL17}. However, these methods fail to perform well under multi-modal demonstrations. To solve this problem, previous work discretizes the continuous action space and learns the action centre through K-means \citep{shafiullah2022behavior}, or adopts implicit policies which formulate imitation as a conditional energy-based modelling (EBM) problem \citep{florence2021implicit}. \citep{chi2023diffusionpolicy} proposes a diffusion model-based policy that handles multi-modality due to the stochastic in both initialization and sampling process of diffusion models~\citep{ho2020denoising}'s stochastic sampling procedure and a stochastic initialization. \citep{robomimic2021} conducts extensive experiments in seek of the leading factors for both behaviour cloning and offline reinforcement learning in robotic manipulation. \\
%%%%%%%%%%%%%%%%%%%%%%%%%%%%%%%%%%%%%%%%%%%%%%%%%%%%%%%%%%%%%%%%%%
\textbf{Representation Learning in Computer Vision.} Learning a generic visual representation that could be fine-tuned for many downstream tasks, including image classification~\citep{Mahajan_2018_ECCV, doersch_2017_iccv}, semantic segmentation~\citep{long_2015_cvpr, Zhao_2017_CVPR}, object detection~\citep{rich_2014_cvpr, doersch2015unsupervised}, has become commonplace in computer vision. There are two dominant categories of methods for learning a representation. One is supervised learning, where ImageNet~\citep{imagenet_cvpr09} classification is the de facto pre-training diagram~\citep{pmlr_v32_donahue14, Razavian2014CNNFO, Kornblith_2019_cvpr, dosovitskiy2021an}. In recent years, to fully exploit large-scale unlabelled data, self-supervised learning (SSL) approaches have been proposed, such as contrastive learning~\citep{he2020momentum, chen2020simple, oord2019representation} or pre-training on pre-text tasks, e.g., reconstruction~\citep{He2021MaskedAA}, Jigsaw puzzles~\citep{Noroozi_2016_eccv} and instance discrimination~\citep{NIPS2014_07563a3f, wu2018unsupervised}. Showing that semantic information is a necessary but not sufficient condition for visuomotor visual pre-training.\\
%%%%%%%%%%%%%%%%%%%%%%%%%%%%%%%%%%%%%%%%%%%%%%%%%%%%%%%%%%%%%%%%%%
\begin{table}[h]
    \centering
\begin{tabular}{ccccc|c}
% \toprule
Policy & \multicolumn{4}{c}{Pre-training} &  \\
\toprule
 & ImageNet & R3M & MVP & VIP & E2E \\
\midrule
BC & 0.15 & 0.236 & 0.122 & 0.116 & 0.657 \\
% \midrule
BC-RNN & 0.337 & 0.489 & nan & 0.125 & 0.657 \\
% \midrule
DP-CNN & nan & 0.679 & 0.776 & 0.263 & 0.938 \\
% \midrule
DP-Trans & nan & 0.673 & 0.682 & 0.269 & nan \\
\bottomrule
\end{tabular}
\caption{pusht}
\label{tab:pusht}
\end{table}

\begin{table}[h]
    \centering
\begin{tabular}{ccccc|c}
Policy & \multicolumn{4}{c}{Pre-training} &  \\
\toprule
 & ImageNet & R3M & MVP & VIP & E2E \\
\midrule
BC & nan & 0.58 & 0.48 & 0.2 & 0.9 \\
BC-RNN & nan & nan & nan & nan & 0.86 \\
DP-CNN & 1.0 & 0.96 & nan & 0.44 & 1.0 \\
DP-Trans & 1.0 & 0.92 & nan & 0.6 & 0.96 \\
\bottomrule
\end{tabular}
\caption{can}
\label{tab:your_label}

\end{table}

\begin{table}[h]
    \centering
\begin{tabular}{ccccc|c}
Policy & \multicolumn{4}{c}{Pre-training} &  \\
\toprule
 & ImageNet & R3M & MVP & VIP & E2E \\
\midrule
BC & nan & 0.36 & 0.34 & 0.02 & 0.8 \\
BC-RNN & 0.62 & 0.66 & nan & nan & 0.92 \\
DP-CNN & 0.76 & 0.78 & nan & 0.04 & 1.0 \\
DP-Trans & 0.86 & 0.72 & nan & 0.2 & 0.92 \\
\bottomrule
\end{tabular}
\caption{stack}
\label{tab:your_label}

\end{table}

\begin{table}[h]
    \centering
\begin{tabular}{ccccc|c}
Policy & \multicolumn{4}{c}{Pre-training} &  \\
\toprule
 & ImageNet & R3M & MVP & VIP & E2E \\
\midrule
BC & nan & 0.2 & 0.12 & nan & 0.52 \\
BC-RNN & 0.6 & nan & nan & nan & 0.76 \\
DP-CNN & nan & 0.52 & nan & 0.06 & 0.92 \\
DP-Trans & 0.74 & 0.5 & nan & 0.16 & 0.88 \\
\bottomrule
\end{tabular}
\caption{square}
\label{tab:your_label}

\end{table}

\begin{table}[h]
    \input{tables/bl_pick_place}
\end{table}

\begin{table}[h]
    \centering
\begin{tabular}{ccccc|c}
Policy & \multicolumn{4}{c}{Pre-training} &  \\
\toprule
 & ImageNet & R3M & MVP & VIP & E2E \\
\midrule
BC & nan & nan & 0.0 & 0.0 & nan \\
BC-RNN & 0.02 & 0.0 & nan & nan & 0.1 \\
DP-CNN & nan & 0.02 & 0.02 & 0.0 & nan \\
DP-Trans & 0.0 & 0.02 & 0.0 & 0.0 & nan \\
\bottomrule
\end{tabular}
\caption{stack\_three}
\label{tab:your_label}

\end{table}

\begin{table}[h]
    \centering
\begin{tabular}{ccccc|c}
Policy & \multicolumn{4}{c}{Pre-training} &  \\
\toprule
 & ImageNet & R3M & MVP & VIP & E2E \\
\midrule
BC & nan & nan & 0.0 & 0.0 & nan \\
BC-RNN & 0.09 & 0.03 & nan & nan & 0.2 \\
DP-CNN & nan & 0.08 & 0.16 & 0.0 & nan \\
DP-Trans & nan & 0.06 & 0.04 & 0.02 & 0.14 \\
\bottomrule
\end{tabular}
\caption{nut\_ass}
\label{tab:your_label}

\end{table}

\begin{table}[ht]
    \centering
    \begin{tabular}{cc|cccc|c}
         & \multicolumn{6}{c}{\textbf{In-domain Pre-trained}}  \\
         \toprule
         \textbf{Task} & \textbf{Policy} & BC & BC-RNN & DP-CNN & DP-Trans & \textbf{E2E} \\
         \midrule
         \multirow{4}{*}{PushT} & BC & -- & 0.47 & 0.30 & \textbf{0.67} & 0.64 \\
         & BC-RNN & 0.74 & -- & 0.78 & \textbf{0.88} & 0.74 \\
         & DP-CNN & 0.82 & 0.79 & -- & 0.86 & \underline{\textbf{0.93}} \\
         & DP-Trans & 0.63 & 0.77 & 0.79 & -- & \textbf{0.89} \\
         \midrule
         \multirow{4}{*}{Can} & BC & -- & \textbf{0.92} & 0.78 & 0.86 & 0.89 \\
         & BC-RNN & 0.90 & -- & 0.97 & \textbf{0.98} & \textbf{0.98} \\
         & DP-CNN & 0.95 & 0.95 & -- & 0.96 & \underline{\textbf{1.00}} \\
         & DP-Trans & 0.82 & 0.87 & 0.95 & -- & \textbf{0.96}\\
         \midrule
         \multirow{4}{*}{Stack} & BC & -- & 0.77 & 0.61 & 0.68 & \textbf{0.78} \\
         & BC-RNN & 0.88 & -- & 0.92 & 0.84 & \textbf{0.96} \\
         & DP-CNN & 0.89 & 0.89 & -- & 0.93 & \underline{\textbf{0.97}} \\
         & DP-Trans & 0.83 & 0.89 & 0.80 & -- & \textbf{0.91} \\
         \midrule
         \multirow{4}{*}{Square} & BC & -- & 0.25 & 0.51 & 0.51 & \textbf{0.52} \\
         & BC-RNN & 0.56 & -- & \textbf{0.86} & 0.84 & 0.69 \\
         & DP-CNN & 0.61 & 0.65 & -- & 0.86 & \underline{\textbf{0.91}} \\
         & DP-Trans & 0.33 & 0.56 & 0.86 & -- & \textbf{0.87} \\
         \bottomrule
    \end{tabular}
    \caption{In-domain pretraining. The empirical results show that end2end training is still dominating under the circumstances of in-domain task-agnostic pretraining of the visual encoder. (300 epochs)}
    \label{tab:exp_indomain}
\end{table}

\begin{figure}[ht]
    \centering
    \small
    \minipage{0.3\textwidth}
    \includegraphics[width=\linewidth]{pics/test_tsne.png}
    \subcaption{}\label{fig:awesome_image1}
    \endminipage\hfill
    \minipage{0.3\textwidth}
        \includegraphics[width=\linewidth]{pics/test_tsne_action.png}
        \subcaption{}\label{fig:awesome_image2}
    \endminipage\hfill
    \vspace{0.3cm}
    \caption{TSNE plot for visual and action distribution of different tasks.}
    \label{fig:enter-label}
\end{figure}
%%%%%%%%%%%%%%%%%%%%%%%%%%%%%%%%%%%%%%%%%%%%%%%%%%%%%%%%%%%%%%%%%%%%%%%
\begin{figure}[ht]
    \centering
    \includegraphics[width=0.5\linewidth]{pics/saliency/imagenet.png}
    \caption{}
    \label{fig:enter-label}
\end{figure}
